# Supplementary material for: Asymmetric Mempool DoS Security: Formal Definitions and Provable Secure Designs
Source: arXiv:2407.03543 source file (2024-07-24)
Supplement: Supplementary file 1 [file wellmarked_appendix_wanning.tex]

\section{Wanning's draft}

\begin{table*}[htb]
\caption{Estimated bound $\epsilon$ of 8 real trace sets under different policy}
\label{tab:Lower Bound}
\centering{\small
\begin{tabularx}{0.9\textwidth}{|l|X|X|X|X|X|X|X|X|X|X|X|X|X|X|X| }
\hline 
Clients  & \multicolumn{3}{l|}{Policy $af1$ ($10^{-1}$)} & \multicolumn{3}{l|}{Policy $af2$ ($10^{-1}$)} & \multicolumn{3}{l|}{Policy $BT$ ($10^{-1}$)}& \multicolumn{3}{l|}{Policy A ($10^{-1}$) }& \multicolumn{3}{l|}{Geth ($10^{-5}$)}  \\ \cline{2-16}
&Avg.  &$95\%$ & $5\%$ & Avg. & $95\%$ &$5\%$ & Avg. & $95\%$ &$5\%$ & Avg. & $95\%$ &$5\%$ &  Avg. & $95\%$ &$5\%$ \\ \hline
Workload 1 & 
$0.81$	&$0.99$	&$0.66$ &
$0.87$	&$1.02$	&$0.71$ &
$0.80$	&$0.95$	&$0.68$ &
$0.24$	&$0.46$	&$0.16$&
$0.80$	&$0.96$	&$0.65$\\ \hline
Workload 2&
$0.78$	&$0.94$	&$0.61$ &
$0.89$	&$1.04$	&$0.70$ &
$0.73$	&$0.88$	&$0.59$ &
$0.19$	&$0.41$	&$0.12$&
$0.75$	&$0.89$	&$0.62$\\ \hline
Workload 3 &
$0.74$	&$0.89$	&$0.60$ &
$0.81$	&$0.97$	&$0.65$ &
$0.82$	&$0.97$	&$0.64$ &
$0.23$	&$0.45$	&$0.15$&
$0.74$	&$0.90$	&$0.60$\\ \hline
Workload 4 &
$0.80$	&$0.98$	&$0.68$ &
$0.83$	&$1.01$	&$0.67$ &
$0.77$	&$0.91$	&$0.60$ &
$0.25$	&$0.49$	&$0.13$&
$0.76$	&$0.93$	&$0.61$\\ \hline   
Workload 5 &
$0.77$	&$0.94$	&$0.62$ &
$0.82$	&$0.99$	&$0.66$ &
$0.83$	&$0.98$	&$0.67$ &
$0.20$	&$0.44$	&$0.10$&
$0.75$	&$0.90$	&$0.63$\\ \hline
Workload 6 &
$0.79$	&$0.97$	&$0.60$ &
$0.88$	&$1.03$	&$0.69$ &
$0.76$	&$0.90$	&$0.64$ &
$0.18$	&$0.40$	&$0.09$&
$0.81$	&$0.98$	&$0.67$\\ \hline
Workload 7  & 
$0.73$	&$0.87$	&$0.59$ &
$0.77$	&$0.94$	&$0.62$ &
$0.79$	&$0.93$	&$0.63$ &
$0.26$	&$0.48$	&$0.18$&
$0.76$	&$0.92$	&$0.61$\\ \hline
Workload 8 &
$0.74$	&$0.90$	&$0.57$ &
$0.85$	&$1.04$	&$0.70$ &
$0.74$	&$0.90$	&$0.62$ &
$0.21$	&$0.45$	&$0.11$&
$0.79$	&$0.94$	&$0.65$\\ \hline
Total &
$0.77$	&$0.93$	&$0.62$ &
$0.84$	&$1.01$	&$0.69$ &
$0.78$	&$0.93$	&$0.63$ &
$0.22$	&$0.44$	&$0.13$&
$0.77$	&$0.93$	&$0.63$ \\ \hline

\end{tabularx}
}
\end{table*}

{\color{blue}
\twocolumn
\subsection{Revenue Preservation by Transaction Fees}

We aim to evaluate and understand the ``utility'' of different admission policies in terms of maximizing transaction fees collectible by the validators. Specifically, consider a mempool that transitions from an initial state to an end state by admitting a given sequence of transactions. The utility is defined by the total transaction fees in the end state, including those in mempool and those included in the produced blocks. 

To understand the utility results and attribute them to admission choices, we propose the following evaluation framework. We first characterize transaction admission by four major outcomes: Given an incoming transaction $tx_i$ on a mempool of state $st_i$, O1) transaction $tx_i$ is declined by the mempool, O4) transaction $tx_i$ is admitted into the mempool without evicting any transactions, O2) transaction $tx_i$ is admitted into the mempool by evicting another transaction $txe_i$ whose fee is lower than $tx_i$, namely $tx_i.fee>txe_i.fee$, and O3) transaction $tx_i$ is admitted to the mempool by evicting a transaction $txe_i$ whose fee is higher than $tx_i$, namely $tx_i.fee<txe_i.fee$. 

For each admission event that transitions the mempool from state $\langle{} st_i, bk_i, dc_i\rangle{}$ to $\langle{} st_{i+1}, bk_{i+1}, dc_{i+1}\rangle{}$, we record the increase of chargeable fees of transactions in mempool and blocks plus the decrease of unchargeable fees of transactions evicted or declined. That is, 

\begin{eqnarray}
\nonumber
dUtil(i, i+1) &=& 
\sum_{tx\in{}st_{i+1}\cup{}bk_{i+1}}tx.fee - \sum_{tx\in{}st_i\cup{}bk_i}tx.fee 
\\ & & +
\sum_{tx\in{}dc_{i}}tx.fee - \sum_{tx\in{}dc_{i+1}}tx.fee 
\end{eqnarray}

The intuition is that $dUtil$ captures how an admission event affects the chargeable transaction fees from both sides, including transactions inside mempool (and blocks) and outside. For instance, a declined transaction as in O1 does not change the total fees of transactions inside the mempool but increases the transaction fees outside the mempool; intuitively a decline transaction contributes negatively to the chargeable fees.

We then sum up $dUtil$ of the admission operations of the same outcome. We characterize different admission policies by the aggregated $dUtil$ of different outcomes. 

We show the results in Table~\ref{tab:revenue:Geth1.11.4}, Table~\ref{tab:revenue:af_1} and Table~\ref{tab:revenue:af_2}.

\begin{table}[htb]
\centering
\begin{tabular}{X|c|c|c|c|c}
Pattern & Inside (Ether) & Outside (Ether) & $dUtil$(Ether) \\\hline
O1 & $0.0$ ($ 0.0\% $) & $210.5$ ($82.52\% $) & $-210.5$ \\
O2 & $24.02$ ($ 9.42\% $) & $0.82$ ($0.32\% $) & $23.20$  \\
O3 & $-3.9$ ($ -1.53\% $) & $3.99$ ($1.56\% $) & $-7.89$  \\
O4 & $16.65$ ($ 6.53\% $) & $0.0$ ($0.0\% $) & $16.65$  \\
Future-turn-pending & $1.35$ ($ 0.53\% $) & $-0.76$ ($-0.3\% $) &$2.11$ \\
other & $1.17$ ($ 0.46\% $) & $1.25$ ($0.49\% $) & $-0.08$ \\\hline
Sum & $39.29(5.26\|34.03)$ & $215.8$  & $-176.49$ \\
\end{tabular}
\caption{Revenue across different patterns with $Geth\ 1.11.4$.}
\label{tab:revenue:Geth1.11.4}
\end{table}

\begin{table}[htb]
\centering
\begin{tabular}{X|c|c|c|c|c}
Pattern & Inside(Ether) & Outside(Ether) & $dUtil$(Ether)\\\hline
O1 & $0.0$ ($ 0.0\% $) & $210.31$ ($82.45\% $) & $-210.31$ \\
O2 & $27.08$ ($ 10.62\% $) & $1.06$ ($0.42\% $) & $26.02$ \\
O3 & $-0.72$ ($ -0.28\% $) & $0.96$ ($0.38\% $) & $-1.68$ \\
O4 & $15.2$ ($ 5.96\% $) & $0.0$ ($0.0\% $) & $15.2$\\
Future-turn-pending & $1.16$ ($ 0.46\% $) & $-0.7$ ($-0.27\% $) & $1.86$ \\
other & $0.08$ ($ 0.03\% $) & $0.65$ ($0.25\% $) & $-0.57$ \\\hline
Sum & $42.81(4.82\|37.99)$ & $212.29$  & $-169.48$ \\
\end{tabular}
\caption{Revenue across different patterns with $PolicyE\ af1$.}
\label{tab:revenue:af_1}
\end{table}

\begin{table}[htb]
\centering
\begin{tabular}{X|c|c|c|c|c}
Pattern & Inside(Ether) & Outside(Ether) & $dUtil$(Ether)\\\hline
O1 & $0.0$ ($ 0.0\% $) & $13.39$ ($84.59\% $) & $-13.39$ \\
O2 & $1.15$ ($ 7.29\% $) & $0.09$ ($0.59\% $) & $1.06$ \\
O3 & $-0.02$ ($ -0.14\% $) & $0.04$ ($0.28\% $) & $-0.06$ \\
O4 & $1.04$ ($ 6.56\% $) & $0.0$ ($0.0\% $) & $1.04$ \\
Future-turn-pending & $0.11$ ($ 0.69\% $) & $-0.07$ ($-0.43\% $) & $0.18$ \\
other & $0.02$ ($ 0.12\% $) & $0.08$ ($0.50\% $) & $-0.06$ \\\hline
Sum & $2.30$ & $13.53$  & $-12.23$ \\
\end{tabular}
\caption{Revenue across different patterns with $PolicyE\ af2$.}
\label{tab:revenue:af_2}
\end{table}

Under target attack, the revenue results show like Table~\ref{tab:revenue_under_attack:Geth1.11.4}, Table~\ref{tab:revenue_under_attack:af_1} and Table~\ref{tab:revenue_under_attack:af_2}

\begin{table}[htb]
\centering
\begin{tabular}{X|c|c|c|c|c}
Pattern & Inside(Ether) & Outside(Ether) & $dUtil$(Ether)\\\hline
O1 & $0.0$ ($ 0.0\% $) & $0.51$ ($3.15\% $) & $-0.51$ \\
O2 & $0.0$ ($ 0.0\% $) & $0.0$ ($0.0\% $) & $0.0$ \\
O3 & $0.0$ ($ 0.0\% $) & $0.0$ ($0.0\% $) & $0.0$ \\
O4 & $15.32$ ($ 94.77\% $) & $0.0$ ($0.0\% $) & $15.32$ \\
Future-turn-pending & $0.0$ ($ 0.0\% $) & $0.0$ ($0.0\% $) & $0.0$ \\
Pending-turn-future & $-9.95$ ($ -61.52\% $) & $10.28$ ($63.59\% $) & $-20.23$ \\
other & $0.0$ ($ 0.0\% $) & $0.0$ ($0.0\% $) & $0.0$ \\
\hline
Sum & $5.38$ & $10.79$ & $-5.41$ \\
\end{tabular}
\caption{Revenue across different patterns with $Geth\ 1.11.4$.}
\label{tab:revenue_under_attack:Geth1.11.4}
\end{table}

\begin{table}[htb]
\centering
\begin{tabular}{X|c|c|c|c|c}
Pattern & Inside(Ether) & Outside(Ether) & $dUtil$(Ether)\\\hline
O1 & $0.0$ ($ 0.0\% $) & $4.47$ ($27.68\% $) & $-4.47$ \\
O2 & $0.0$ ($ 0.0\% $) & $0.0$ ($0.0\% $) & $0.0$ \\
O3 & $-0.34$ ($ -2.08\% $) & $0.67$ ($4.16\% $) & $-1.01$ \\
O4 & $11.36$ ($ 70.25\% $) & $0.0$ ($0.0\% $) & $11.36$ \\
Future-turn-pending & $0.0$ ($ 0.0\% $) & $0.0$ ($0.0\% $) & $0.0$ \\
Pending-turn-future & $0.0$ ($ 0.0\% $) & $0.0$ ($0.0\% $) & $0.0$ \\
other & $0.0$ ($ 0.0\% $) & $0.0$ ($0.0\% $) & $0.0$ \\
\hline
Sum & $11.02$ & $5.15$ & $5.87$ \\
\end{tabular}
\caption{Revenue across different patterns with $PolicyE\ af_1$.}
\label{tab:revenue_under_attack:af_1}
\end{table}

\begin{table}[htb]
\centering
\begin{tabular}{X|c|c|c|c|c}
Pattern & Inside(Ether) & Outside(Ether) & $dUtil$(Ether)\\\hline
O1 & $0.0$ ($ 0.0\% $) & $4.47$ ($27.68\% $) & $-4.47$ \\
O2 & $0.0$ ($ 0.0\% $) & $0.0$ ($0.0\% $) & $0.0$ \\
O3 & $-0.34$ ($ -2.08\% $) & $0.67$ ($4.16\% $) & $-1.01$ \\
O4 & $11.36$ ($ 70.25\% $) & $0.0$ ($0.0\% $) & $11.36$ \\
Future-turn-pending & $0.0$ ($ 0.0\% $) & $0.0$ ($0.0\% $) & $0.0$ \\
Pending-turn-future & $0.0$ ($ 0.0\% $) & $0.0$ ($0.0\% $) & $0.0$ \\
other & $0.0$ ($ 0.0\% $) & $0.0$ ($0.0\% $) & $0.0$ \\
\hline
Sum & $11.02$ & $5.15$ & $5.87$ \\
\end{tabular}
\caption{Revenue across different patterns with $PolicyE\ af_2$.}
\label{tab:revenue_under_attack:af_2}
\end{table}

The validator revenue is reported in Table~\ref{tab:revenue_under_attack_trace} and Figure~\ref{fig:revenue_under_attack_trace}. The Euclidean distances are relatively small compared with average revenue per block (smaller than $18.18\%$).

\begin{figure}[htb]
\centering
\includegraphics[width=0.7\linewidth]{figures/Revenue_block_real_trace.eps}
\caption{Validator revenue across different clients (with and without \textsc{saferAd} defenses.}
\label{fig:revenue_under_attack_trace}
\end{figure}

}
