# Supplementary material for: Asymmetric Mempool DoS Security: Formal Definitions and Provable Secure Designs
Source: arXiv:2407.03543 source file (2024-07-24)
Supplement: Supplementary file 2 [file wellmarked_appendix_yibo.tex]

{\color{blue}{
\section{Maximal-Gas assumption validation}

This section validates the maximal-Gas assumption 
%(A2 as described in \S~\ref{sec:background}) 
on leading Ethereum execution-layer clients including Geth, Besu, Erigon and Flashbot Builder.

We specifically test these clients under two properties: A2a) When finishing building a block, Algorithm $\textsc{bdBk}()$ has tried but failed at inserting {\it any} transaction in the current mempool to the block due to the block Gas exceeding Limit $g_b$. A2b) When trying to add a mempool transaction to a block, Algorithm $\textsc{bdBk}()$ tries {\it only} appending the transaction to the last position in the block and does not try other positions.

Evaluation of A2a: As shown in Figure~\ref{fig:assumptiona}, in test case $TC 1$, we set up a mempool with $3$ transactions, $Tx1$ with high price (e.g., $5$ Gwei) and $21,000$ Gas, $Tx2$ with medium price (e.g., $8$ Gwei) and $30M - 1$ Gas and $Tx3$ with low price (e.g., $5$ Gwei) and $21,000$ Gas. We observe $Tx1$ and $Tx3$ are included in the next generated block $B_i$. To validate that Algorithm $\textsc{bdBk}()$ has tried to add $Tx2$ but fails due to exceeding block Gas limit $30M$, we design a differential experiment in test case $TC 2$. In $TC 2$, given the same mempool setup as $TC 1$, we customize the block Gas limit to $30M + 42000$ Gas. We observe $Tx1$, $Tx2$ and $Tx3$ are all included in next block $B_i$. 

We set up an Ethereum execution-layer client and a validator running on top of it (e.g., Prysm in consensus-layer) in a local environment. We send $Tx1$, $Tx2$ and $Tx3$ with the setting of $TC 1$ and $TC 2$ respectively as described above. In all the tested clients, the block $B_i$ generated next includes $Tx1$ and $Tx3$ in $TC 1$ and all $Tx1$, $Tx2$ and $Tx3$ in $TC 2$.

\begin{figure}[!ht]
  \centering
    \subfloat[Assumption A2a]{%
  \includegraphics[width=0.2\textwidth]{figures/assumptiona.eps}%
  \label{fig:assumptiona}}
\subfloat[Assumption A2b]{%
  \includegraphics[width=0.266\textwidth]{figures/assumptionb.eps}%
\label{fig:assumptionb}}%
\caption{Assumption test case.}
\end{figure}
Evaluation of A2b: As shown in Figure~\ref{fig:assumptionb}, given a mempool with 2 transactions, say $Tx1$ and $Tx2$, Algorithm $\textsc{bdBk}()$ orders the transactions in {$Tx1$, $Tx2$} in test case $TC 1$. We observe only $Tx1$ is included in the next block. To validate that Algorithm $\textsc{bdBk}()$ does not try to insert $Tx2$ before $Tx1$, we design a differential experiment in test case $TC 2$. When transactions are ordered in {$Tx2$, $Tx1$} in $TC 2$, we observe that both $Tx2$, $Tx1$ are included in the next block. The experiment result shows if $Tx2$ is executed before $Tx1$, both transactions can be included in blocks. However, given a specific transaction order (e.g., price descending order), Algorithm $\textsc{bdBk}()$ only tries to add transactions to the last position of the block by following the order.

In our experiment, $Tx1$ is a smart contract invocation calling function foo() in the smart contract ValidateA2b as shown in Figure~\ref{lst:validationsmartcontract}. When the state variable $a$ is in the initial state, executing foo() costs $30M - 1$ Gas. $Tx2$ calls function bar() to update the state variable “a” to $0$. As a result, executing foo() after bar() only costs $2,200$ Gas. We assume the transactions are ordered in price descending order. In $TC 1$, $Tx1$ is with high price (e.g., $10$ Gwei) and $Tx2$ is low price (e.g., $5$ Gwei). In contrast, the prices of $Tx1$ and $Tx2$ are low and high price respectively in $TC 2$. 

\input{text/lst15_varification.tex}

We set up an Ethereum execution-layer client and a validator running on top of it (e.g., Prysm in consensus-layer) in a local environment. We send $Tx1$ and $Tx2$ with the setting of $TC 1$ and $TC 2$ respectively as described above. In all the tested clients, the block $B_i$ generated next only includes $Tx1$ in $TC 1$ and both $Tx1$ and $Tx2$ in $TC 2$.

}}
