# Supplementary material for: Asymmetric Mempool DoS Security: Formal Definitions and Provable Secure Designs
Source: arXiv:2407.03543 source file (2024-07-24)
Supplement: Supplementary file 3 [file appendix.tex]

\input{text/paper25-wellappendix}

%\clearpage {\color{blue}\input{text/buffer}}

%\clearpage \input{text/wanning-proof}

%\clearpage \input{text/appendix25.tex}
%\input{text/wellmarked_appendix23.tex}
%wellmarked_appendix31.tex
